# Supplementary material for: On the performance of high-order finite elements with respect to maximum principles and the non-negative constraint for diffusion-type equations
Source: arXiv:1108.0952 source file (2011-08-03)
Supplement: Supplementary file 1 [file LS_DMP_Appendix.tex]

%*****************************************;
%                                         ;
%  NAME                                   ;
%    LS_DMP_Appendix.tex                  ;
%                                         ;
%*****************************************;
\section*{APPENDIX}
\label{Sec:LS_DMP_Appendix}
We now present the finite element ``stiffness'' matrices and 
``load'' vectors in two popular notations. The first one is 
using Kronecker products, and the other one is using the 
standard Voigt notation. 

%========================================;
%  Subsection: Using Kronecker products  ;
%========================================;
\subsection{Using Kronecker products}

%====================================;
%  Subsection: Using Voigt notation  ;
%====================================;
\subsection{Using Voigt notation}
In both formulations, the finite element equations for a
typical element may be expressed as

\begin{equation}
\left[ {\begin{array}{*{20}{c}}
   {{{\mathbf{K}}^{11}}} & {{{\mathbf{K}}^{12}}} & {{{\mathbf{K}}^{13}}}  \\
   {{{\mathbf{K}}^{21}}} & {{{\mathbf{K}}^{22}}} & {{{\mathbf{K}}^{23}}}  \\
   {{{\mathbf{K}}^{31}}} & {{{\mathbf{K}}^{32}}} & {{{\mathbf{K}}^{33}}}  \\
\end{array} } \right]\left\{ {\begin{array}{*{20}{c}}
   {\mathbf{u}}  \\
   {{{\mathbf{q}}_{\mathbf{x}}}}  \\
   {{{\mathbf{q}}_{\mathbf{y}}}}  \\
\end{array} } \right\} = \left\{ {\begin{array}{*{20}{c}}
   {{{\mathbf{F}}^1}}  \\
   {{{\mathbf{F}}^1}}  \\
   {{{\mathbf{F}}^2}}  \\
\end{array} } \right\}
\label{eq18}
\end{equation}

\noindent In least-squares formulation 1, the components of the coefficient matrices
$ K_{ij}^{\alpha \beta } $ are of the form

\begin{equation}
\begin{split}
  K_{ij}^{11} &= \int_{{\Omega ^e}} {\left[ {{\alpha ^2}S_{ij}^{00} + \left( {D_{xy}^2 + D_{xx}^2} \right)S_{ij}^{11} + \left( {D_{xy}^2 + D_{yy}^2} \right)S_{ij}^{22} + {{\tilde D}_{xy}}\left( {S_{ij}^{12} + S_{ij}^{21}} \right)} \right]dxdy}  \hfill \\
  K_{ij}^{12} &= K_{ji}^{21} = \int_{{\Omega ^e}} {\left( {\alpha S_{ij}^{01} + {D_{xx}}S_{ij}^{10} + {D_{xy}}S_{ij}^{20}} \right)dxdy}  \hfill \\
  K_{ij}^{13} &= K_{ji}^{31} = \int_{{\Omega ^e}} {\left( {\alpha S_{ij}^{02} + {D_{xy}}S_{ij}^{10} + {D_{yy}}S_{ij}^{20}} \right)dxdy}  \hfill \\
  K_{ij}^{22} &= \int_{{\Omega ^e}} {\left( {S_{ij}^{00} + S_{ij}^{11}} \right)dxdy}  \hfill \\
  K_{ij}^{23} &= K_{ji}^{32} = \int_{{\Omega ^e}} {S_{ij}^{12}dxdy}  \hfill \\
  K_{ij}^{33} &= \int_{{\Omega ^e}} {\left( {S_{ij}^{00} + S_{ij}^{22}} \right)dxdy}  \hfill
\end{split}
\label{eq19}
\end{equation}

\noindent where $ {\tilde D_{xy}} = {D_{xy}}\left( {{D_{xx}} + {D_{yy}}} \right) $.
Likewise in least-squares formulation 2, the components of $ K_{ij}^{\alpha \beta } $ may be
expressed as

\begin{equation}
\begin{split}
  K_{ij}^{11} &= \int_{{\Omega ^e}} {\left[ {{\alpha ^2}S_{ij}^{00} + {D_{xx}}S_{ij}^{11} + {D_{yy}}S_{ij}^{22} + {D_{xy}}\left( {S_{ij}^{12} + S_{ij}^{21}} \right)} \right]dxdy}  \hfill \\
  K_{ij}^{12} &= K_{ji}^{21} = \int_{{\Omega ^e}} {\left( {\alpha S_{ij}^{01} + S_{ij}^{10}} \right)dxdy}  \hfill \\
  K_{ij}^{13} &= K_{ji}^{31} = \int_{{\Omega ^e}} {\left( {\alpha S_{ij}^{02} + S_{ij}^{20}} \right)dxdy}  \hfill \\
  K_{ij}^{22} &= \int_{{\Omega ^e}} {\left( {S_{ij}^{11} + D_{xx}^{ - 1}S_{ij}^{00}} \right)dxdy}  \hfill \\
  K_{ij}^{23} &= K_{ji}^{32} = \int_{{\Omega ^e}} {\left( {S_{ij}^{12} + D_{xy}^{ - 1}S_{ij}^{00}} \right)dxdy}  \hfill \\
  K_{ij}^{33} &= \int_{{\Omega ^e}} {\left( {S_{ij}^{22} + D_{yy}^{ - 1}S_{ij}^{00}} \right)dxdy}  \hfill \\
\end{split}
\label{eq20}
\end{equation}

\noindent In both formulations the components of the force vector $ F_i^\alpha $ are of the
form

\begin{equation}
F_i^1 = \int_{{\Omega ^e}} {\alpha f{\psi _i}dxdy} ,\quad \quad F_i^2 = \int_{{\Omega ^e}} {f\frac{{\partial {\psi _i}}}
{{\partial x}}dxdy} ,\quad \quad F_i^3 = \int_{{\Omega ^e}} {f\frac{{\partial {\psi _i}}}
{{\partial y}}dxdy}
\label{eq21}
\end{equation}

\noindent In the above expressions we have utilized the following definitions

\begin{equation}
\begin{gathered}
  S_{ij}^{00} = {\psi _i}{\psi _j}, {\kern 73.75pt} S_{ij}^{11} = \frac{{\partial {\psi _i}}}
{{\partial x}}\frac{{\partial {\psi _j}}}
{{\partial x}} \hfill \\
  S_{ij}^{22} = \frac{{\partial {\psi _i}}}
{{\partial y}}\frac{{\partial {\psi _j}}}
{{\partial y}}, {\kern 55.25pt} S_{ij}^{01} = S_{ji}^{10} = {\psi _i}\frac{{\partial {\psi _i}}}
{{\partial x}} \hfill \\
  S_{ij}^{12} = S_{ji}^{21} = \frac{{\partial {\psi _i}}}
{{\partial x}}\frac{{\partial {\psi _i}}}
{{\partial y}}, \quad \quad S_{ij}^{02} = S_{ji}^{20} = {\psi _i}\frac{{\partial {\psi _i}}}
{{\partial y}} \hfill \\
\end{gathered}
\label{eq22}
\end{equation}
